# Supplementary material for: SVG-IR: Spatially-Varying Gaussian Splatting for Inverse Rendering
Source: arXiv:2504.06815 source file (2025-04-09)
Supplement: Supplementary file 1 [file sec_X-supplementary.tex]

\clearpage
\setcounter{page}{1}
\maketitlesupplementary

We propose SVG-IR, a novel inverse rendering framework based on our proposed Spatially-varying Gaussian representation with spatially-varying material attributes. Besides we introduce our physically-based illumination to better decouple material properties and illumination.
In this supplementary material, we provide implementation details \cref{sec:imple_details}, along with additional results \cref{sec:sup_res} and ablation study \cref{sec:sup_ab}.

\section{Implementation details}
\label{sec:imple_details}
\paragraph{Spatially-varying Gaussian representation.}

As described in \cref{sec:CG}. In our Spatially-varying Gaussian, we define several Gaussian vertices with different material attributes on a single Gaussian primitive. The Gaussian vertices are parameterized on the tangent space of each Gaussian defined by the rotation matrix $R$ and the scaling matrix $S$. In implementation, we create a square on each Gaussian surfel, where the length of each side of the square is determined by twice the scaling $S$ along the two axes.

\paragraph{Ray tracing.}
We perform ray tracing on Gaussian surfels in \cref{sec:pbi} to obtain the incoming radiance of each Gaussian. When constructing the BVH, we treat each Gaussian as an elliptical disk, where the lengths of the two axes are set to three times the scaling factor, and the thickness of each disk is defined as $1 \times 10^{-12}$. We perform uniform sample on the up hemisphere of each Gaussian $K$ ($K$=64 in our experiments) times to get $K$ sampled directions. For each Gaussian, we emit rays along the $K$ sampled directions as well as along the upper hemisphere to perform ray intersections. When a ray hits a Gaussian, the new ray's starting point is the hit point, plus an offset of $\epsilon$ (set as 0.05) times the ray direction, and the ray tracing continues from there. The radiance and transmittance are accumulated as \eqref{eq:radiance_ind} and \eqref{eq:trans}. The ray tracing results are stored in the micro-buffers of each Gaussian for later direct queries, eliminating the need to re-trace the rays. 
Besides, during ray tracing, we also record the index $I$ of the first Gaussian hit and its coordinates in the tangent space $U$, which are stored in the Gaussian's buffer as well.
\paragraph{One-bounce indirect illumination.}
\label{sec:impl_one-bounce}
We replace the indirect illumination from the radiance colors of Gaussians with one-bounce indirect illumination in \cref{sec:relighting}. Thanks to the micro-buffers stored in ray-tracing, we can utilize the index buffers $I$ to query the bounce between Gaussians quickly with the tangent space coordinates $U$ to determine the weights of interpolation. Then we can compute the one-bounce indirect illumination in \eqref{eq:one-bounce} with a fast speed.

\paragraph{Radiance consistency loss.}
We leverage one-bounce indirect illumination as a supervision when training by sampling the specular direction as
\begin{equation}
    k_j = \mathrm{argmax}(<\omega_o^k, 2\boldsymbol{N}_o^g-\omega_i> \And V_j^k=0) 
\end{equation}
where $\omega_o^k$ represents the view direction on Gaussian $j$. 
We only sample on directions that are not visible to direct light, ensuring the presence of indirect lighting from bounces between Gaussians. Thus, We can compute the radiance consistency loss as \eqref{eq:rad_loss}. As described in \cref{sec:impl_one-bounce}, the index micro buffers also reduce the computation time this loss less than 1 ms.

\paragraph{Loss details.}

We train Gaussian vertex attributes using loss terms in \eqref{eq:loss}.
% \begin{equation}
% \begin{split}
%     \mathcal{L}=&\lambda_{1} \mathcal{L}_{1}+\lambda_{\text{ssim}} \mathcal{L}_{\text{ssim}}+\lambda_{\text{rad}} \mathcal{L}_{\text{rad}} \\
%     &\lambda_{n} \mathcal{L}_{n}+\lambda_{s, a} \mathcal{L}_{s, a}+\lambda_{s, r} \mathcal{L}_{s, r}+\lambda_{\mathrm{reg},n} \mathcal{L}_{\mathrm{reg},n},
%     \end{split}
% \end{equation}
The $\mathcal{L}_{1}$ and $\mathcal{L}_{\text{ssim}}$ reprensent $L_1$ loss and SSIM loss between rendered image and ground truth, which are commonly used rendering loss by previous methods~\cite{kerbl_2023_3dgs, liang_2024_gsir, gao_2023_relightablegs}. $\mathcal{L}_{\text{ec}}$ is the radiance consistency loss defined in \eqref{eq:rad_loss}. $\mathcal{L}_{s, a}$ is TV-loss on albedo for smoothness, defined as
\begin{equation}
    \begin{split}
        \Delta_{ij}^{\hat{\mathbf{\alpha}}}=&\exp\left(-|I_{i,j}-I_{i-1,j}|\right)(\hat{\mathbf{\alpha}}_{i,j}-\hat{\mathbf{\alpha}}_{i-1,j})^{2}+\\
        &\exp\left(-|I_{i,j}-I_{i,j-1}|\right)(\hat{\mathbf{\alpha}}_{i,j}-\hat{\mathbf{\alpha}}_{i,j-1})^{2}, \\
        \mathcal{L}_{s, a}=&\frac{1}{|\hat{\mathbf{\alpha}}|}\sum_{i,j}\Delta_{ij}^{\hat{\mathbf{\alpha}}},
    \end{split}
\end{equation}
where $\hat{\mathbf{\alpha}}$ is the albedo map obtained by the SVG splatting in \cref{sec:CG-IR}. $\mathcal{L}_{s, r}$ is the TV-loss on roughness similar to $\mathcal{L}_{s, a}$. $\mathcal{L}_{n}$ is the normal consistency loss in Gaussian surfels~\cite{dai_2024_gaussiansurfels} by
\begin{equation}
    \mathcal{L}_n=(1-\hat{n}^\top\hat{n}_{\hat{D}})
\end{equation}
where $\hat{n}$ is normal map and $\hat{n}_{\hat{D}}$ is the pseudo normal map from the depth map. $\mathcal{L}_{\mathrm{reg},n}$ is $L_2$ regular term of normal offsets from Gaussian Shader~\cite{Jiang24GaussianShader} as
\begin{equation}
    \mathcal{L}_{\mathrm{reg},n} = ||\Delta{N}^{\{M\}}||^2
\end{equation}
The loss weights $\{\lambda_{1}, \lambda_{\text{ssim}}, \lambda_{\text{rc}}, \lambda_{n}, \lambda_{s,a}, \lambda_{s,r}, \lambda_{reg, n}\}$ are set as $\{0.9, 0.1, 0.05, 0.02, 0.1, 0.05, 0.01\}$.

\section{More results}
\label{sec:sup_res}
\paragraph{Results on TensoIR Synthetic dataset.}
\label{sec:res_tensoir}
We show more inverse rendering results on Figs.~\ref{fig:sup_armadillo} to~\ref{fig:sup_lego}. The metrics on albedo and normal are shown in Tab.~\ref{tab:sup_mat}. Relightable 3DGS~\cite{gao_2023_relightablegs} conducts over-smooth normal and albedo. GaussianShader~\cite{Jiang24GaussianShader} produces unnatural relighting results. Due to the residual color terms and the approximation of PBR. GS-IR~\cite{liang_2024_gsir} produces coarse normals and albedo with baked-in lighting effects. TensoIR~\cite{jin_2023_tensoir} lacks the details in rendering, e.g. the texture on the bread in the hotdog scene. Our method leverages Spatially-varying Gaussians and physically-based illumination to enhance representational capacity and lighting decoupling, achieving high-quality results on both relighting and NVS. We also provide detailed per-scene results in Tab.~\ref{tab:sup_tensoir_others}.

% Table generated by Excel2LaTeX from sheet 'Sheet2'
\begin{table}[t]
  \centering
  \footnotesize
  \caption{Comparison of albedo and normal on TensoIR Synthetic and ADT datasets. Numbers in \sotacolor{red} represent the best performance, while \subsotacolor{orange} numbers denote the second best.}
  \resizebox{0.85\linewidth}{!}{
  
    \begin{tabular}{c|lc@{\hskip 1.5pt}c@{\hskip 1.5pt}c@{\hskip 1.5pt}c@{\hskip 1.5pt}cc}
    \hline
    \multirow{8}[6]{*}{\rotatebox{90}{TensoIR}} & \multicolumn{1}{c}{\multirow{2}[2]{*}{Method}} & \multicolumn{5}{c}{Albedo}            & Normal \\
          &       & PSNR$\uparrow$  & /     & SSIM$\uparrow$  & /     & LPIPS$\downarrow$ & MAE$\downarrow$ \\
\cline{2-8}          & MII   & 27.293 & /     & 0.933 & /     & 0.101 & 5.076 \\
          & TensoIR & 29.275 & /     & \subsotacolor{0.950} & /     & 0.087 & \sotacolor{4.098} \\
          & Gsshader & 25.026 & /     & 0.923 & /     & 0.087 & 5.757 \\
          & GS-IR & \subsotacolor{30.286} & /     & 0.941 & /     & \subsotacolor{0.084} & 5.341 \\
          & RelightGS & 28.537 & /     & 0.922 & /     & 0.087 & 5.064 \\
\cline{2-8}          & Ours  & \sotacolor{30.341} & /     & \sotacolor{0.951} & /     & \sotacolor{0.074} & \subsotacolor{4.358} \\
    \hline
    \multirow{6}[4]{*}{\rotatebox{90}{ADT}} & MII   & 29.150 & /     & 0.952 & /     & 0.068 & 3.027 \\
          & TensoIR & 29.295 & /     & 0.954 & /     & 0.056 & 2.688 \\
          & Gsshader & 30.432 & /     & 0.960  & /     & \subsotacolor{0.036} & \subsotacolor{1.995} \\
          & GS-IR & \subsotacolor{32.711} & /     & \subsotacolor{0.968} & /     & 0.037 & 2.665 \\
          & RelightGS & 21.047 & /     & 0.911 & /     & 0.039 & 2.179 \\
\cline{2-8}          & Ours  & \sotacolor{33.630} & /     & \sotacolor{0.980} & /     & \sotacolor{0.023} & \sotacolor{1.703} \\
    \hline
    \end{tabular}%
    }
  \label{tab:sup_mat}%
\end{table}%

\paragraph{Results on ADT dataset.}
\label{sec:res_adt}
We show more inverse rendering results on Figs.~\ref{fig:sup_airplane} to~\ref{fig:sup_Gargoyle}. The metrics on albedo and normal are shown in Tab.~\ref{tab:sup_mat}. We achieve excellent inverse rendering and relighting results thanks to our SVG-IR framework in ADT dataset. We also provide detailed per-scene results in Tab.~\ref{tab:sup_adt_others}.

\paragraph{Results on DTU dataset.}
\label{sec:res_dtu}
In Fig.~\ref{fig:sup_dtu}, we demonstrate the inverse rendering results of our method on the real-world DTU dataset~\cite{jensen2014large}. Utilizing our SVG-IR framework, we recover the material properties and achieve high-quality relighting. Besides, our approach produces natural indirect lighting, thanks to our physically-based illumination model.

\paragraph{Results on NeILF++ dataset.}
\label{sec:res_neilfpp}
To verify its robustness in relighting, we further evaluate our method on the real-world dataset NeILF++~\cite{zhang_2023_neilfpp}, scomparing it against GS-IR~\cite{Liang24GS-IR} and Relightable 3DGS~\cite{gao_2023_relightablegs}, as shown in Fig.~\ref{fig:sup_neilfpp}. The results demonstrate the robustness of our SVG-IR framework, achieving high-quality relighting even on the relatively sparse-view real-world dataset.

\paragraph{Results on Mip-NeRF360 dataset.}
\label{sec:res_mip}
Fig.~\ref{fig:sup_mip} showcases the inverse rendering and relighting results of our method on MipNeRF360 datasets~\cite{barron_2022_mipnerf360}. Our SVG-IR framework achieves high-quality reconstruction with the Spatially-varying Gaussian and physically-based illumination, demonstrating robust performance on scene-level real-world datasets.

% Table generated by Excel2LaTeX from sheet 'Sheet1'
\begin{table}[t]
  \centering
  \caption{Comparison of NVS quality between our method and others on NeRF Synthetic dataset. \sotacolor{Red} numbers represent the best performance, and \subsotacolor{orange} denotes the second best.}
  \resizebox{\linewidth}{!}{
    \begin{tabular}{lcccc}
    \toprule
    Method & Relightable & PSNR↑ & SSIM↑ & LPIPS↓ \\
    \midrule
    NeRF~\cite{mildenhall_2020_nerf}  & \ding{55}     & 31.012 & 0.947 & 0.056 \\
    Plenoxels~\cite{fridovich_2022_plenoxels} & \ding{55}     & 31.714 & 0.958 & 0.053 \\
    TensoRF~\cite{chen_2022_tensorf} & \ding{55}     & \subsotacolor{33.140} & \subsotacolor{0.963} & 0.042 \\
    3DGS~\cite{kerbl_2023_3dgs}  & \ding{55}     & \sotacolor{33.883} & \sotacolor{0.971}  & \sotacolor{0.031} \\
    GaussianSurfels~\cite{dai_2024_gaussiansurfels} & \ding{55}     & 33.053 & 0.961  & \subsotacolor{0.036} \\
    \midrule
    TensoIR~\cite{jin_2023_tensoir} & \ding{51}     & 29.537 & 0.943 & 0.067 \\
    GaussianShader~\cite{Jiang24GaussianShader} & \ding{51}     & \sotacolor{33.367} & \sotacolor{0.960}  & \sotacolor{0.042} \\
    RelightGS~\cite{gao_2023_relightablegs} & \ding{51}     & 28.238 & 0.938 & 0.056 \\
    GS-IR~\cite{liang_2024_gsir} & \ding{51}     & 30.133 & 0.937 & 0.059 \\
    Ours  & \ding{51}     & \subsotacolor{30.338} & \subsotacolor{0.946} & \subsotacolor{0.051} \\
    \bottomrule
    \end{tabular}%
    }
  \label{tab:sup_nerf}%
\end{table}%

\paragraph{Results on NeRF Synthetic dataset.}
\label{sec:res_nerf}
We evaluate the NVS performance of our method on the NeRF Synthetic dataset~\cite{mildenhall_2020_nerf} and compare it with both relightable and non-relightable approaches in Tab.~\ref{tab:sup_nerf}. Among relightable methods, our approach achieves near SOTA NVS quality. GaussianShader builds upon the radiance SH representation in 3DGS by incorporating BRDF, rather than replacing radiance SH with BRDF as other methods do. This enables it to achieve the NVS quality comparable to the original 3DGS at the expense of relighting performance. In contrast, our Spatially-varying Gaussian representation and physically-based illumination enable competitive NVS quality while preserving relighting fidelity.

\paragraph{Results of normal and albedo in ablation study.}

\hanxiao{The impact of Spatially-varying Gaussian (SVG), visibility (Vis.), and indirect ill. (Ind.) on the normal and albedo quality is in Tab.~\ref{tab:re_ab}.}

\begin{table}[htbp]
  \centering
  \vspace{-9px}
  \caption{Nor./albedo quality in ablation study (TensoIR dataset). }
  \vspace{-8px}
  %CG is the Spatially-varying Gaussian representation, ``Vis.'' is the visibility and ``Ind.'' is the indirect illumination.}
  \resizebox{0.8\linewidth}{!}{
    \begin{tabular}{rrrcccc}
    \toprule
    \multicolumn{3}{c}{Component} & \multicolumn{3}{c}{Albedo} & Normal \\
    \midrule
    \multicolumn{1}{c}{SVG} & \multicolumn{1}{c}{Vis.} & \multicolumn{1}{c}{Ind.} & PSNR↑ & SSIM↑ & LPIPS↓ & MAE ↓ \\
    \midrule
    \ding{55}      &    \ding{55}   &    \ding{55}   & 26.84 & 0.926 & 0.099 & 4.77 \\
    \ding{51}     &    \ding{55}   &    \ding{55}   & 27.94 & 0.931 & 0.080  & 4.53 \\
    \ding{51}     & \ding{51}     &    \ding{55}   & 29.26 & 0.945 & \textbf{0.073} & 4.39 \\
    \ding{51}     & \ding{51}     & \ding{51}     & \textbf{30.34} & \textbf{0.951} & 0.074 & \textbf{4.36} \\
    \bottomrule
    \end{tabular}%
    }
    \vspace{-10px}
  \label{tab:re_ab}%
\end{table}%

\paragraph{Results of R3DG combined with 2D Gaussian.}
\hanxiao{We combine R3DG with 2DGS, similar to our method, and compare it to R3DG, and ours in Tab.~\ref{tab:re_r3dg_2d}.
While R3DG(2D) shows an improvement in relighting quality compared to R3DG, it is 1.2dB lower than ours due to its limited representation capacity and lack of physical constraints for indirect illumination.}

\begin{table}[htbp]
  \centering
  \caption{R3DG vs. R3DG(2D) vs. ours (TensoIR dataset).
  %The results of replace the 3D Gaussians of Relightable 3DGS with 2D Gaussians on TensoIR dataset.
  }
  \vspace{-8px}
  \resizebox{\linewidth}{!}{
\begin{tabular}{lccccc}
    \toprule
    \multicolumn{1}{l}{\multirow{2}[2]{*}{Method}} & Gaussian & Relight & NVS   & Albedo & Normal \\
          &  Count &  PSNR↑ &  PSNR ↑ &  PSNR ↑ &  MAE ↓ \\
    \midrule
    R3DG  & $\sim$ 20k  & 27.60  & 33.35 & 28.54 & 5.06 \\
    R3DG(2D) & $\sim$ 14k  & 28.96 & 32.82 & 29.25 & 4.72 \\
    Ours  & $\sim$ 14k  & \textbf{31.10}  & \textbf{36.71}& \textbf{30.34} & \textbf{4.36} \\
    \bottomrule
    \end{tabular}%
    
    }
    \vspace{-10px}
    
  \label{tab:re_r3dg_2d}%
\end{table}%

\section{More ablation study}
\label{sec:sup_ab}

% \begin{table}[htbp]
%   \centering
%   \caption{Ablation study of our key components on TensoIR Synthetic dataset. ``CG'' means the Curved Gaussian representation, ``PBI'' means the physically-based illumination. Numbers in \sotacolor{red} represent the best performance, while \subsotacolor{orange} numbers denote the second best.}
%   \resizebox{\linewidth}{!}{
%     \begin{tabular}{rrcccccc}
%     \toprule
%     \multicolumn{2}{c}{Component} & \multicolumn{3}{c}{Relighting} & \multicolumn{3}{c}{NVS} \\
%     \midrule
%     \multicolumn{1}{c}{CG} & \multicolumn{1}{c}{PBI} & PSNR↑ & SSIM↑ & LPIPS↓ & PSNR↑ & SSIM↑ & LPIPS↓ \\
%     \midrule
%     \ding{55}      &   \ding{55}    & 28.614 & 0.904 & 0.093 & 34.640 & 0.941 & 0.047 \\
%     \ding{51}     &  \ding{55}     & \subsotacolor{29.447} & \subsotacolor{0.937} & \subsotacolor{0.074} & \subsotacolor{35.794} & \subsotacolor{0.961} & \subsotacolor{0.041} \\
%     \ding{51}     & \ding{51}     & \sotacolor{31.087} & \sotacolor{0.946} & \sotacolor{0.055} & \sotacolor{36.709} & \sotacolor{0.975} & \sotacolor{0.033} \\
%     \bottomrule
%     \end{tabular}%
%     }
%   \label{tab:ab_key}%
%   %\vspace{-8pt}
% \end{table}%

% Table generated by Excel2LaTeX from sheet 'Sheet1'

\paragraph{Loss.}

\begin{table}[t]
  \centering
  \caption{Ablation study of the loss terms. Numbers in \sotacolor{red} represent the best performance, while \subsotacolor{orange} numbers denote the second best.}
  \resizebox{\linewidth}{!}{
    \begin{tabular}{rrrcccccc}
    \toprule
    \multicolumn{3}{c}{Component} & \multicolumn{3}{c}{Relighting} & \multicolumn{3}{c}{NVS} \\
    \midrule
    \multicolumn{1}{c}{$\mathcal{L}_N$} & \multicolumn{1}{c}{$\mathcal{L}_s$} & \multicolumn{1}{c}{ $\mathcal{L}_{rc}$} & PSNR↑ & SSIM↑ & LPIPS↓ & PSNR↑ & SSIM↑ & LPIPS↓ \\
    \midrule
       \ding{55}   & \ding{51}     & \ding{51}     & 30.002 & 0.939 & 0.062 & 36.379 & 0.972 & \subsotacolor{0.034} \\
    \ding{51}     &    \ding{55}   & \ding{51}     & \subsotacolor{30.753} & 0.941 & \sotacolor{0.054} & \sotacolor{36.722} & \subsotacolor{0.975} & 0.035 \\
    \ding{51}     & \ding{51}     &   \ding{55}    & 30.662 & \subsotacolor{0.943} & 0.061 & 36.444 & 0.974 & 0.035 \\
    \ding{51}     & \ding{51}     & \ding{51}     & \sotacolor{31.087} & \sotacolor{0.946} & \subsotacolor{0.055} & \subsotacolor{36.709} & \sotacolor{0.975} & \sotacolor{0.033} \\
    \bottomrule
    \end{tabular}%
    }
  \label{tab:sup_ab_loss}%
\end{table}%

% We conduct ablation experiments on losses to analysis the impact of the losses. We separate losses in~\cref{sec:trainingdetails} into three categories. First is normal loss $\mathcal{L}_N$ including $\mathcal{L}_n$. Second is smooth loss $\mathcal{L}_s$ including $\mathcal{L}_{s,a}$ and $\mathcal{L}_{s,r}$. Third is our proposed radiance consistency loss $\mathcal{L}_{rad}$.
We perform ablation experiments on the loss functions to analyze their impact. The loss terms outlined in~\cref{sec:imple_details} are divided into three categories: (1) the normal loss $\mathcal{L}_N$, which includes $\mathcal{L}_n$; (2) the smoothness loss $\mathcal{L}_s$, comprising $\mathcal{L}_{s,a}$ and $\mathcal{L}_{s,r}$; and (3) our proposed radiance consistency loss $\mathcal{L}_{rc}$. The metrics are shown in Tab.~\ref{tab:sup_ab_loss}. Normals require constraints to prevent overfitting due to their inherent ambiguity in appearance representation. Smooth loss terms on material parameters lead to cleaner rendering results than those without such regularization, which is beneficial for relighting. 
The radiance consistency loss leverages the pre-trained radiance field to provide supervision from additional viewpoints, improving the quality of both relighting and NVS.

\paragraph{Ray sample counts and cost.}
We conduct additional experiments on the counts of the sampled directions for per Gaussian. We evaluate the quality, memory cost and rendering time on ``armadillo'' from TensoIR Synthetic as shown in Tab~\ref{tab:sup_ab_sample}. Under the observation that the quality reaches a plateau at $K=64$, while maintaining real-time rendering speed and acceptable memory usage, we finally select $K=64$ for the balance of the quality and the cost.

\begin{table}[t]
  \centering
  \caption{Ablation on the sample counts. We present the relighting quality and corresponding cost at different sample counts $K$. Numbers in \sotacolor{red} represent the best performance, while \subsotacolor{orange} numbers denote the second best. In practice, we set $K=64$.}
  \resizebox{\linewidth}{!}{
    \begin{tabular}{cccccccc}
    \toprule
    \multicolumn{3}{c}{\multirow{2}[4]{*}{Sample count}} & \multicolumn{3}{c}{Relighting} & \multicolumn{2}{c}{Cost} \\
\cmidrule{4-8}    \multicolumn{3}{c}{}  & PSNR↑ & SSIM↑ & LPIPS↓ & Memory↓ & Rendering Time↓ \\
    \midrule
    \multicolumn{3}{c}{$K=16$} & 34.114 & 0.9587 & 0.05627 & \sotacolor{11.1GB} & \sotacolor{10ms} \\
    \multicolumn{3}{c}{$K=32$} & 34.842 & 0..96112 & 0.05542 & \subsotacolor{12.1GB} & \subsotacolor{11ms} \\
    \multicolumn{3}{c}{$K=64$} & \sotacolor{35.010} & \subsotacolor{0..96289} & \subsotacolor{0.05401} & 14.3GB & 13ms \\
    \multicolumn{3}{c}{$K=128$} & \subsotacolor{35.009} & \sotacolor{0.96311} & \sotacolor{0.05392} & 20.4GB & 21ms \\
    \bottomrule
    \end{tabular}%
    }
  \label{tab:sup_ab_sample}%
\end{table}%

\begin{figure}[t]
    \centering
    \includegraphics[width=\linewidth]{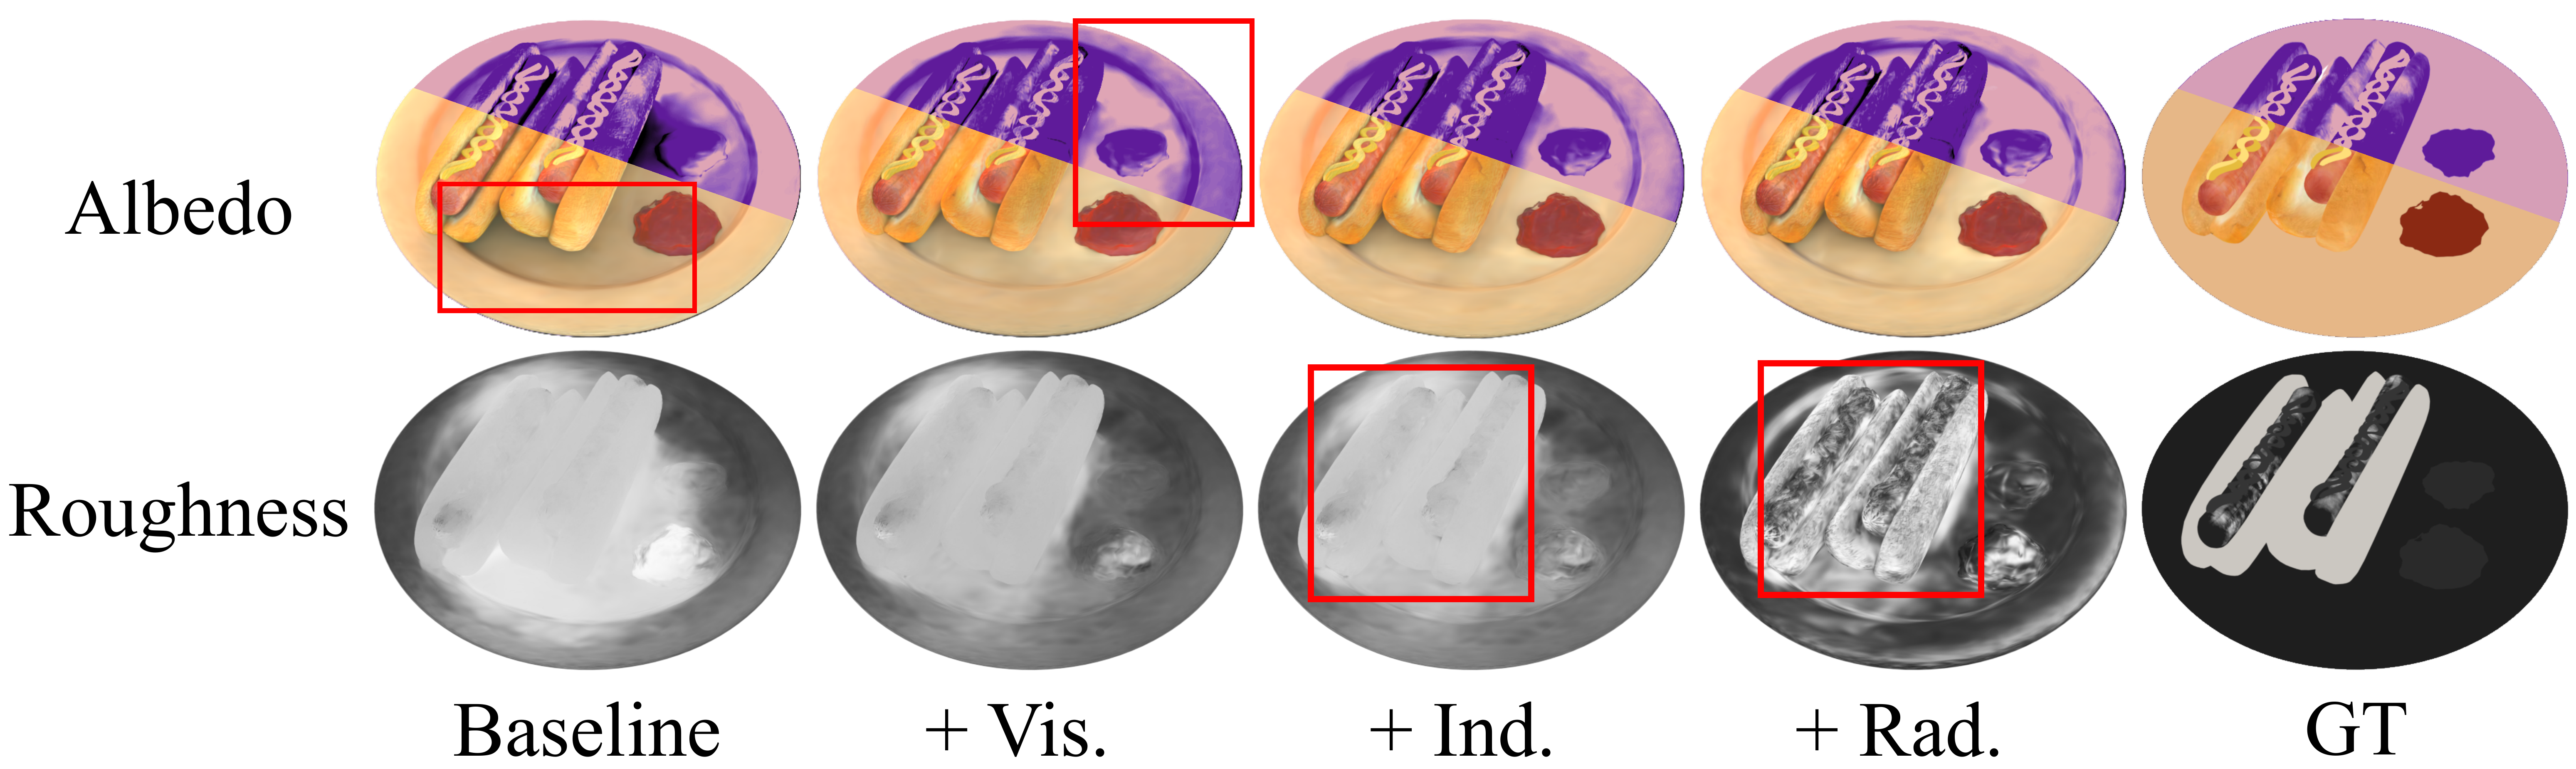}
    \caption{Ablation of indirect illumination components and radiance consistency loss. ``Vis." means the visibility, ``Ind." means the indirect illumination and ``Rad." means the radiance consistency loss. The right part of albedo maps are processed with higher contrast for better observation. The GT roughness is from the ``hotdog'' blender scene in NeRF Synthetic dataset~\cite{mildenhall_2020_nerf} rather than the TensoIR dataset.~\cite{jin_2023_tensoir}}
    \label{fig:ab_ii}
  %  \vspace{-14pt}
\end{figure}

\paragraph{Indirect illumination.}
Fig.~\ref{fig:ab_ii} presents the ablation results for albedo and roughness maps. By modeling visibility, we alleviate the issue of shadows being baked into the albedo in baseline methods. Indirect illumination modeling further helps decoupling of material and lighting, preventing discrepancies in albedo caused by differing lighting conditions from the left to right. Moreover, indirect illumination serves as the foundation of our proposed radiance consistency loss $\mathcal{L}_{rad}$, which ensures roughness aligns more closely with the ground truth. This improvement is achieved through the additional viewpoint guidance provided by $\mathcal{L}_{rad}$.

\paragraph{Gaussian vertex count.}

\hanxiao{As shown in Tab.~\ref{tab:re_ab_number}, more Gaussian vertices result in higher quality with more storage. We choose M=4 in our experiments as a trade-off. }

\begin{table}[htbp]
  \centering
  \caption{Ablation study on GV count (TensoIR dataset). Red dot means a GV. Lagrange interpolation is used.  
  %The red dots on the black ellipse represent the positions of vertices on the Gaussian. 
  }
  \vspace{-8px}
  \resizebox{0.85\linewidth}{!}{
  
    \begin{tabular}{llcccc}
    \toprule
    \multicolumn{2}{c}{Vertex} & Relight & NVS   & Albedo & Normal \\
    Count & Distrib. &  PSNR↑ &  PSNR ↑ &  PSNR ↑ &  MAE ↓ \\
    \midrule
    M = 2  & \begin{minipage}{0.002\textwidth}
       \includegraphics[width=30px]{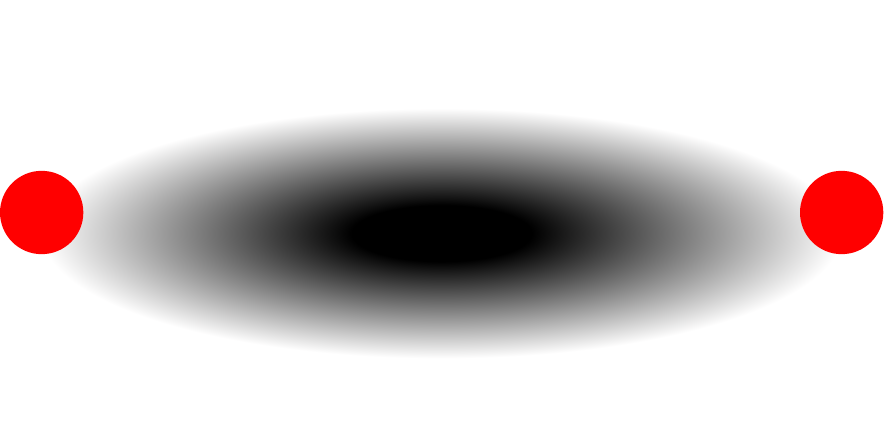}
    \end{minipage}  & 30.01  & 36.37  & 28.02  & 4.90 \\
    M = 4 & \begin{minipage}{0.002\textwidth}
       \includegraphics[width=30px]{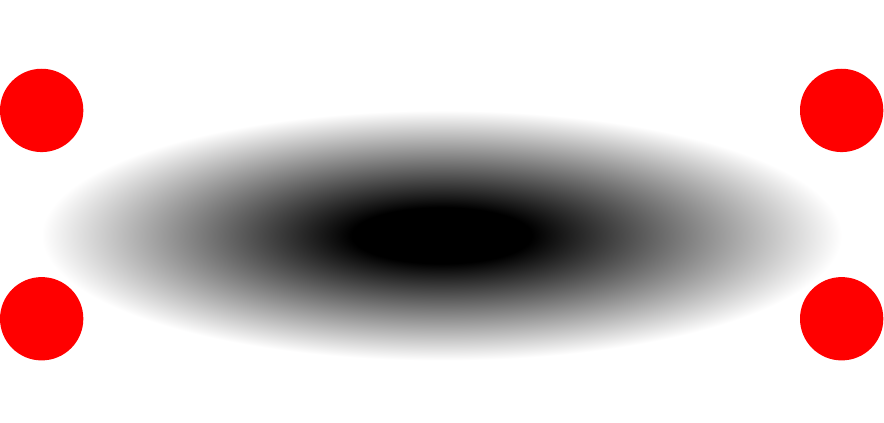}
    \end{minipage}  & 31.10  & 36.71  & 30.34  & 4.36 \\
    M = 6  & \begin{minipage}{0.002\textwidth}
       \includegraphics[width=30px]{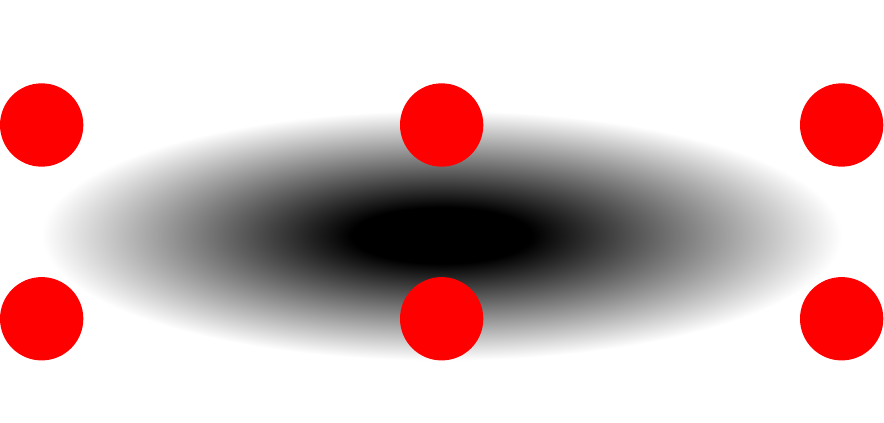}
    \end{minipage}  & \textbf{31.17}  & \textbf{36.77}  & \textbf{30.74}  & \textbf{4.33} \\
 %   M = 8  & \begin{minipage}{0.002\textwidth}
%       \includegraphics[width=30px]{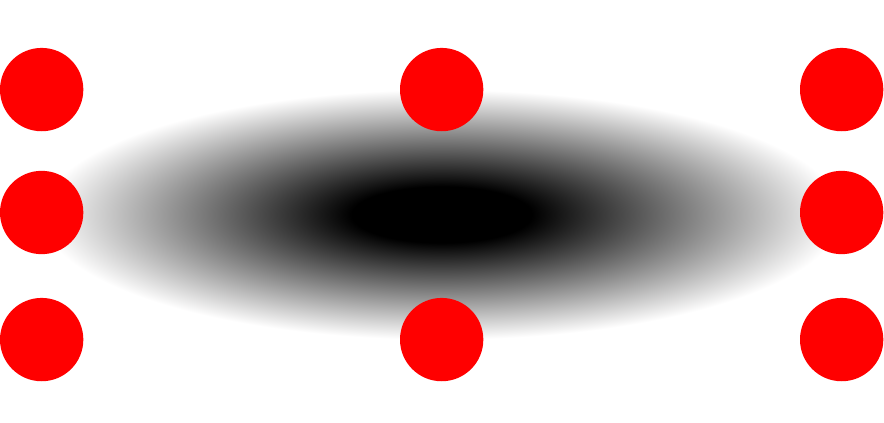}
%    \end{minipage}  & 31.13  & 36.89  & 30.66  & 4.32 \\
    \bottomrule
    \end{tabular}%
    }
  \label{tab:re_ab_number}%
  \vspace{-10px}
\end{table}%

\begin{table*}[htbp]
  \centering
  \footnotesize
  \caption{Per-scene results of normal, albedo and NVS on TensoIR Synthetic dataset. For albedo results, we follow NeRFactor~\cite{zhang_2021_nerfactor} by scaling each RGB channel by a global scalar.}
  \resizebox{0.8\textwidth}{!}{ % 调整表格到页面宽度
  
    \begin{tabular}{cc|c|ccc|ccc}
    \hline
    \multirow{2}[2]{*}{Scene} & \multicolumn{1}{c|}{\multirow{2}[2]{*}{Method}} & Normal & \multicolumn{3}{c|}{Albedo} & \multicolumn{3}{c}{Novel View Synthesis} \\
          &       & MAE$\downarrow$  & PSNR$\uparrow$  & SSIM$\uparrow$  & LPIPS$\downarrow$ & PSNR$\uparrow$  & SSIM$\uparrow$  & LPIPS$\downarrow$ \\
    \hline
    \multirow{6}[2]{*}{Armadillo} & InvRender & 1.732 & 35.573 & 0.959 & 0.076 & 36.681 & 0.971 & 0.056 \\
          & TensoIR & 1.960 & 34.360 & 0.989 & 0.059 & 39.070 & 0.986 & 0.039 \\
          & GSshader & 2.107 & 31.092 & 0.938 & 0.053 & 42.445 & 0.989 & 0.024 \\
          & GS-IR & 3.105 & 38.572 & 0.986 & 0.051 & 38.530 & 0.972 & 0.041 \\
          & RelightGS & 2.224 & 34.435 & 0.933 & 0.067 & 39.440 & 0.980 & 0.042 \\
          & Ours  & 1.974 & 36.851 & 0.973 & 0.047 & 41.057 & 0.983 & 0.031 \\
    \hline
    \multirow{6}[2]{*}{Ficus} & InvRender & 4.884 & 25.335 & 0.942 & 0.072 & 25.498 & 0.939 & 0.062 \\
          & TensoIR & 4.400 & 27.130 & 0.964 & 0.044 & 29.770 & 0.973 & 0.041 \\
          & GSshader & 4.513 & 28.239 & 0.966 & 0.028 & 35.256 & 0.990 & 0.012 \\
          & GS-IR & 5.104 & 30.867 & 0.948 & 0.053 & 33.258 & 0.960 & 0.039 \\
          & RelightGS & 4.991 & 28.597 & 0.912 & 0.057 & 32.405 & 0.974 & 0.028 \\
          & Ours  & 3.408 & 31.580 & 0.972 & 0.032 & 34.899 & 0.978 & 0.025 \\
    \hline
    \multirow{6}[2]{*}{Hotdog} & InvRender & 3.708 & 27.028 & 0.950 & 0.094 & 32.219 & 0.952 & 0.070 \\
          & TensoIR & 4.050 & 30.370 & 0.947 & 0.099 & 36.780 & 0.976 & 0.046 \\
          & GSshader & 8.315 & 18.149 & 0.909 & 0.127 & 36.897 & 0.980 & 0.029 \\
          & GS-IR & 4.774 & 26.745 & 0.941 & 0.088 & 34.843 & 0.969 & 0.051 \\
          & RelightGS & 5.399 & 25.277 & 0.939 & 0.087 & 30.371 & 0.943 & 0.045 \\
          & Ours  & 4.016 & 27.252 & 0.952 & 0.078 & 36.329 & 0.977 & 0.034 \\
    \hline
    \multirow{6}[2]{*}{Lego} & InvRender & 9.980 & 21.435 & 0.882 & 0.160 & 28.277 & 0.887 & 0.133 \\
          & TensoIR & 5.980 & 25.240 & 0.900 & 0.145 & 35.040 & 0.970 & 0.033 \\
          & GSshader & 8.094 & 22.625 & 0.877 & 0.140 & 35.403 & 0.976 & 0.024 \\
          & GS-IR & 8.380 & 24.958 & 0.889 & 0.143 & 33.455 & 0.954 & 0.042 \\
          & RelightGS & 7.643 & 25.838 & 0.902 & 0.135 & 30.371 & 0.943 & 0.045 \\
          & Ours  & 8.032 & 25.681 & 0.901 & 0.139 & 34.551 & 0.964 & 0.041 \\
    \hline
    \end{tabular}%
    }
  \label{tab:sup_tensoir_others}%
\end{table*}%

% Table generated by Excel2LaTeX from sheet 'Sheet2'
\begin{table*}[htbp]
  \centering
  \footnotesize
  \caption{Per-scene results of normal, albedo and NVS on ADT dataset. For albedo results, we follow NeRFactor~\cite{zhang_2021_nerfactor} by scaling each RGB channel by a global scalar.}
    \resizebox{0.8\textwidth}{!}{ % 调整表格到页面宽度
  
        \begin{tabular}{cc|c|ccc|ccc}
    \hline
    \multirow{2}[2]{*}{Scene} & \multicolumn{1}{c|}{\multirow{2}[2]{*}{Method}} & Normal & \multicolumn{3}{c|}{Albedo} & \multicolumn{3}{c}{Novel View Synthesis} \\
          &       & MAE $\downarrow$  & PSNR$\uparrow$  & SSIM$\uparrow$  & LPIPS$\downarrow$ & PSNR$\uparrow$  & SSIM$\uparrow$  & LPIPS$\downarrow$ \\
    \hline
    \multirow{6}[2]{*}{Airplane} & InvRender & 1.688 & 30.240 & 0.978 & 0.037 & 32.794 & 0.985 & 0.022 \\
          & TensoIR & 1.320 & 32.400 & 0.983 & 0.022 & 40.370 & 0.995 & 0.011 \\
          & GSshader & 1.207 & 33.233 & 0.974 & 0.024 & 44.640 & 0.997 & 0.004 \\
          & GS-IR & 1.584 & 35.449 & 0.978 & 0.035 & 38.755 & 0.985 & 0.020 \\
          & RelightGS & 1.298 & 35.375 & 0.973 & 0.034 & 37.982 & 0.991 & 0.01 \\
          & Ours  & 0.876 & 36.172 & 0.987 & 0.017 & 42.568 & 0.994 & 0.007 \\
    \hline
    \multirow{6}[1]{*}{Birdhouse} & InvRender & 3.912 & 27.770 & 0.948 & 0.107 & 31.237 & 0.943 & 0.076 \\
          & TensoIR & 2.960 & 29.350 & 0.961 & 0.084 & 39.350 & 0.986 & 0.031 \\
          & GSshader & 3.148 & 25.984 & 0.929 & 0.061 & 42.167 & 0.990 & 0.016 \\
          & GS-IR & 4.811 & 28.466 & 0.944 & 0.057 & 37.057 & 0.977 & 0.033 \\
          & RelightGS & 3.083 & 25.245 & 0.939 & 0.055 & 36.935 & 0.982 & 0.027 \\
          & Ours  & 2.911 & 29.674 & 0.963 & 0.04  & 40.395 & 0.987 & 0.019 \\
    \hline
    \multirow{6}[1]{*}{Gargoyle} & InvRender & 2.982 & 29.064 & 0.924 & 0.066 & 29.874 & 0.945 & 0.054 \\
          & TensoIR & 3.310 & 28.430 & 0.923 & 0.067 & 39.050 & 0.993 & 0.010 \\
          & GSshader & 1.616 & 30.846 & 0.972 & 0.024 & 42.497 & 0.996 & 0.004 \\
          & GS-IR & 1.711 & 31.955 & 0.973 & 0.022 & 35.904 & 0.984 & 0.013 \\
          & RelightGS & 2.253 & 31.424 & 0.931 & 0.025 & 38.910 & 0.989 & 0.007 \\
          & Ours  & 1.581 & 35.09 & 0.989 & 0.012 & 42.079 & 0.995 & 0.005 \\
    \hline
    \multirow{6}[2]{*}{Calculator} & InvRender & 3.526 & 29.526 & 0.956 & 0.061 & 29.854 & 0.954 & 0.050 \\
          & TensoIR & 3.160 & 27.000 & 0.949 & 0.051 & 40.100 & 0.993 & 0.016 \\
          & GSshader & 2.007 & 31.665 & 0.965 & 0.036 & 43.857 & 0.996 & 0.005 \\
          & GS-IR & 2.553 & 34.973 & 0.976 & 0.032 & 37.470 & 0.983 & 0.022 \\
          & RelightGS & 2.081 & 27.216 & 0.948 & 0.042  & 33.915 & 0.986 & 0.013 \\
          & Ours  & 1.445 & 33.582 & 0.980  & 0.021 & 40.881 & 0.993 & 0.009 \\
    \hline
    \end{tabular}%
   }
  \label{tab:sup_adt_others}%
\end{table*}%

\mycfiguret{sup_armadillo}{sup_armadillo.pdf}{Qualitative comparison of NVS, normal, albedo and relighting on \textbf{armadillo} of TensoIR Synthetic dataset.}
\mycfiguret{sup_ficus}{sup_ficus.pdf}{Qualitative comparison of NVS, normal, albedo and relighting on \textbf{ficus} of TensoIR Synthetic dataset. }
\mycfiguret{sup_hotdog}{sup_hotdog.pdf}{Qualitative comparison of NVS, normal, albedo and relighting on \textbf{hotdog} of TensoIR Synthetic datasets. }
\mycfiguret{sup_lego}{sup_lego.pdf}{Qualitative comparison of NVS, normal, albedo and relighting on \textbf{lego} of TensoIR Synthetic dataset. }

\mycfiguret{sup_airplane}{sup_airplane.pdf}{Qualitative comparison of NVS, normal, albedo and relighting on \textbf{airsplane} of ADT dataset. }
\mycfiguret{sup_birdhouse}{sup_birdhouse.pdf}{Qualitative comparison of NVS, normal, albedo and relighting on \textbf{birdhouse} of ADT dataset. }
\mycfiguret{sup_calculator}{sup_calculator.pdf}{Qualitative comparison of NVS, normal, albedo and relighting on \textbf{calculator} of ADT dataset. }
\mycfiguret{sup_Gargoyle}{sup_Gargoyle.pdf}{Qualitative comparison of NVS, normal, albedo and relighting on \textbf{Gargoyle} of ADT dataset. }

% \begin{figure*}[t]
%     \vspace{-20pt}
%     \centering
%     \includegraphics[width=0.95\textwidth]{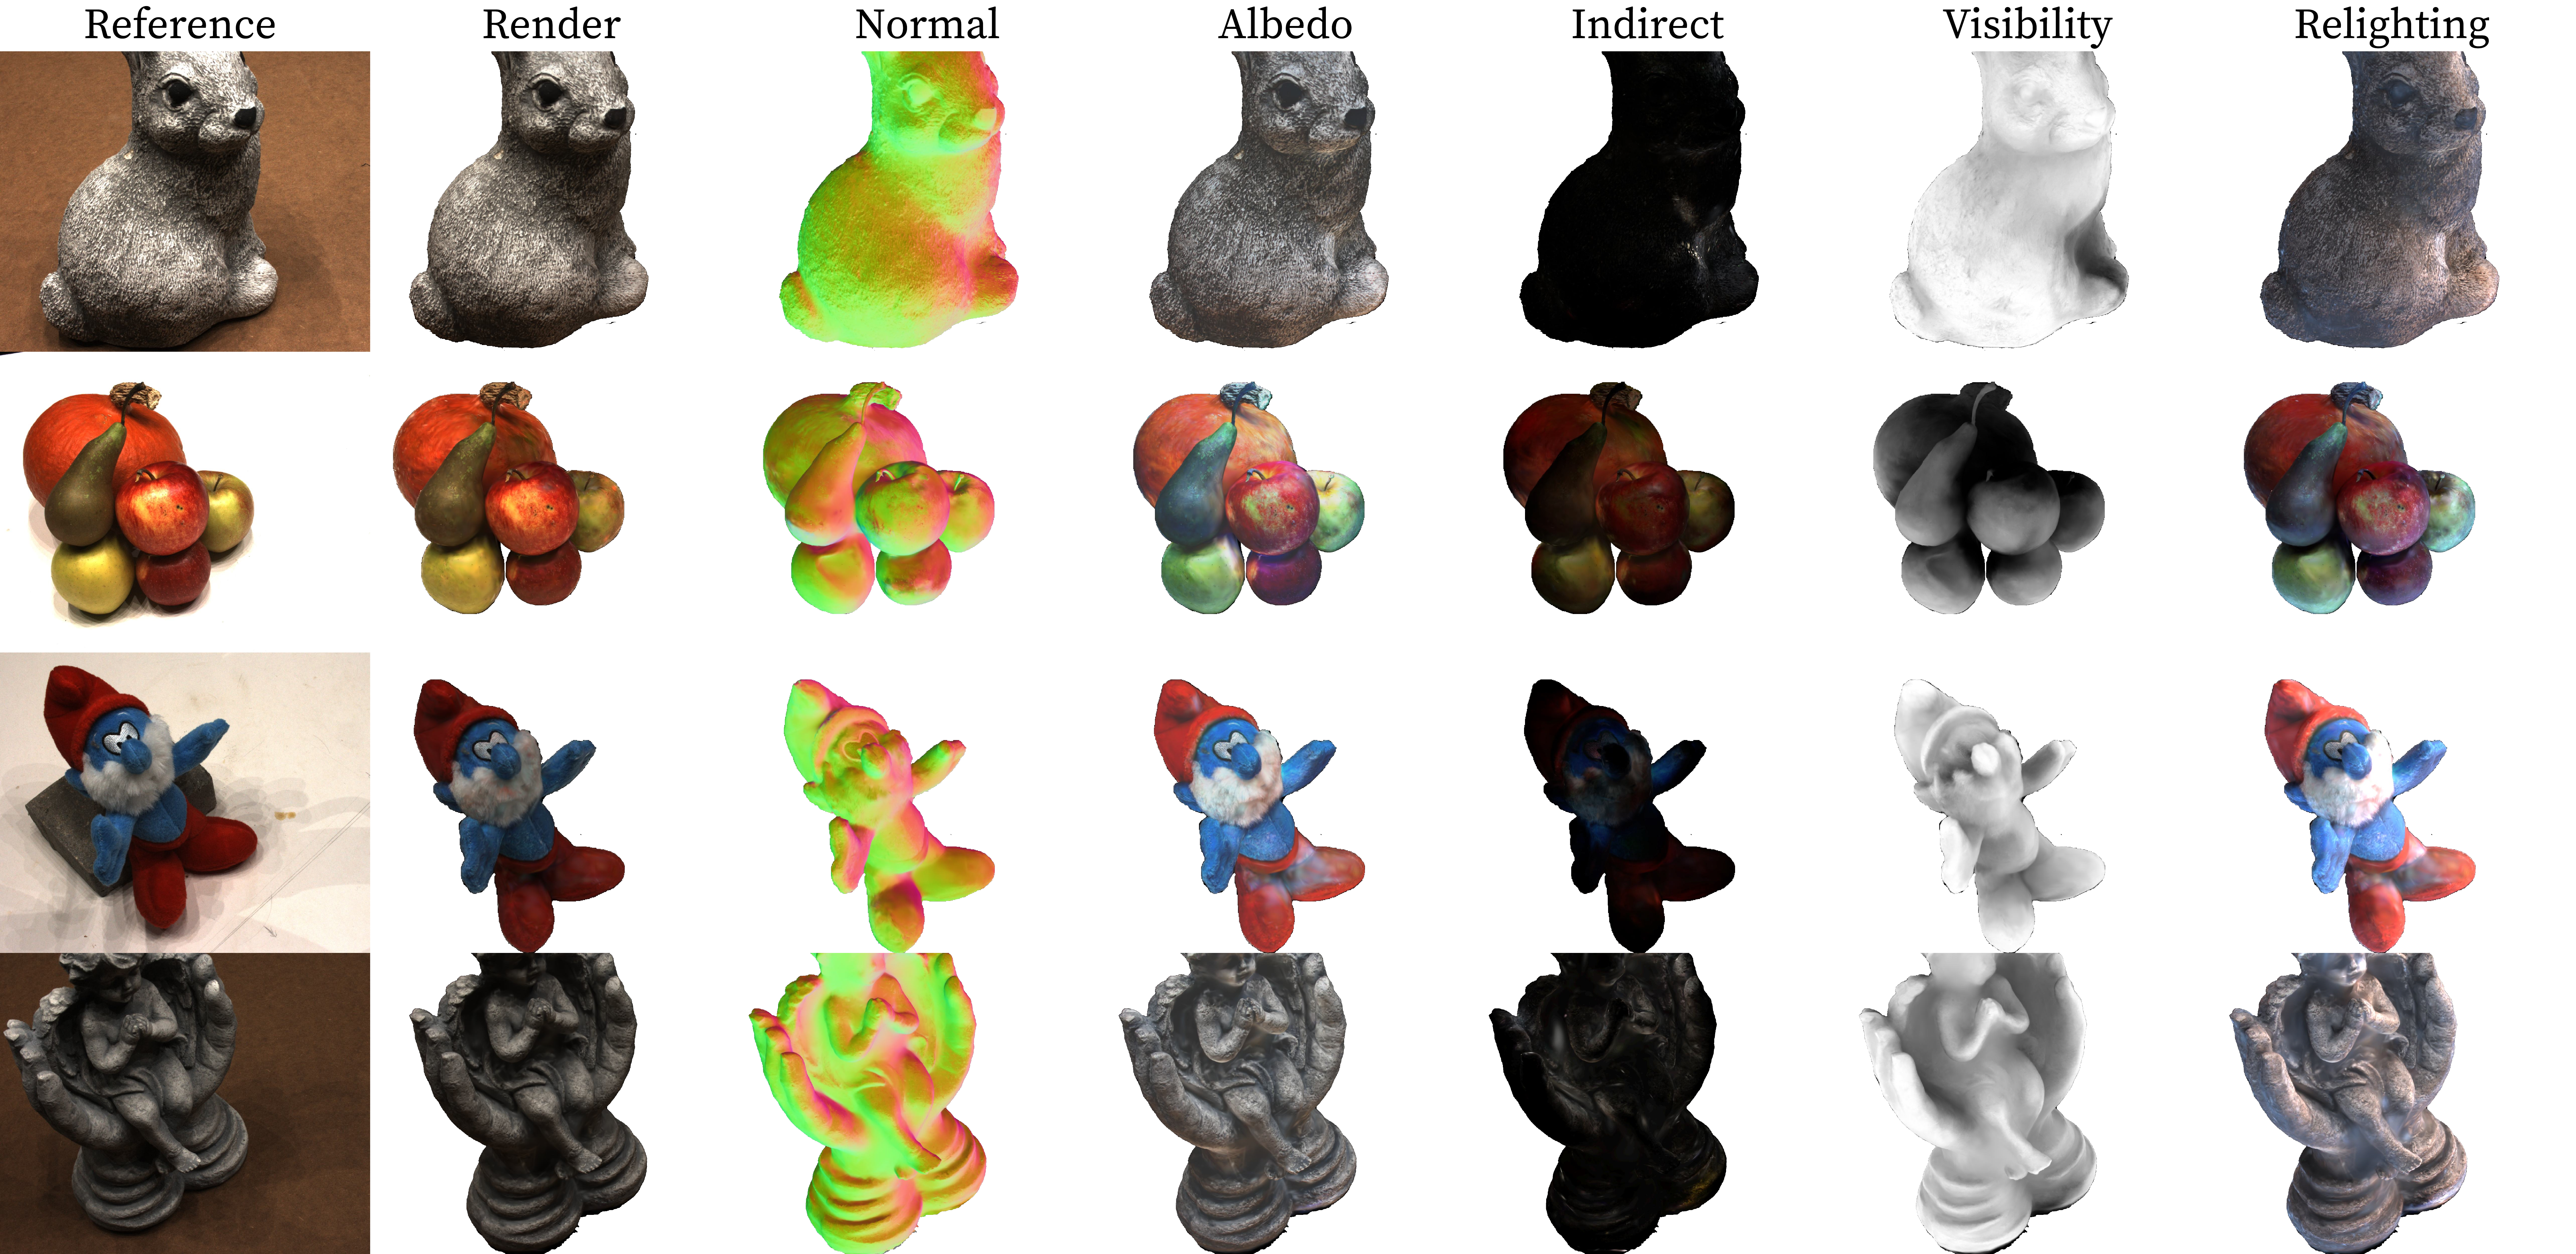}
%     \caption{Inverse rendering and relighting results on DTU dataset.}
%     \label{fig:sup_dtu}
%     \vspace{-20pt}
% \end{figure*}

% \begin{figure*}[t]
%     \vspace{-20pt}
%     \centering
%     \includegraphics[width=0.95\textwidth]{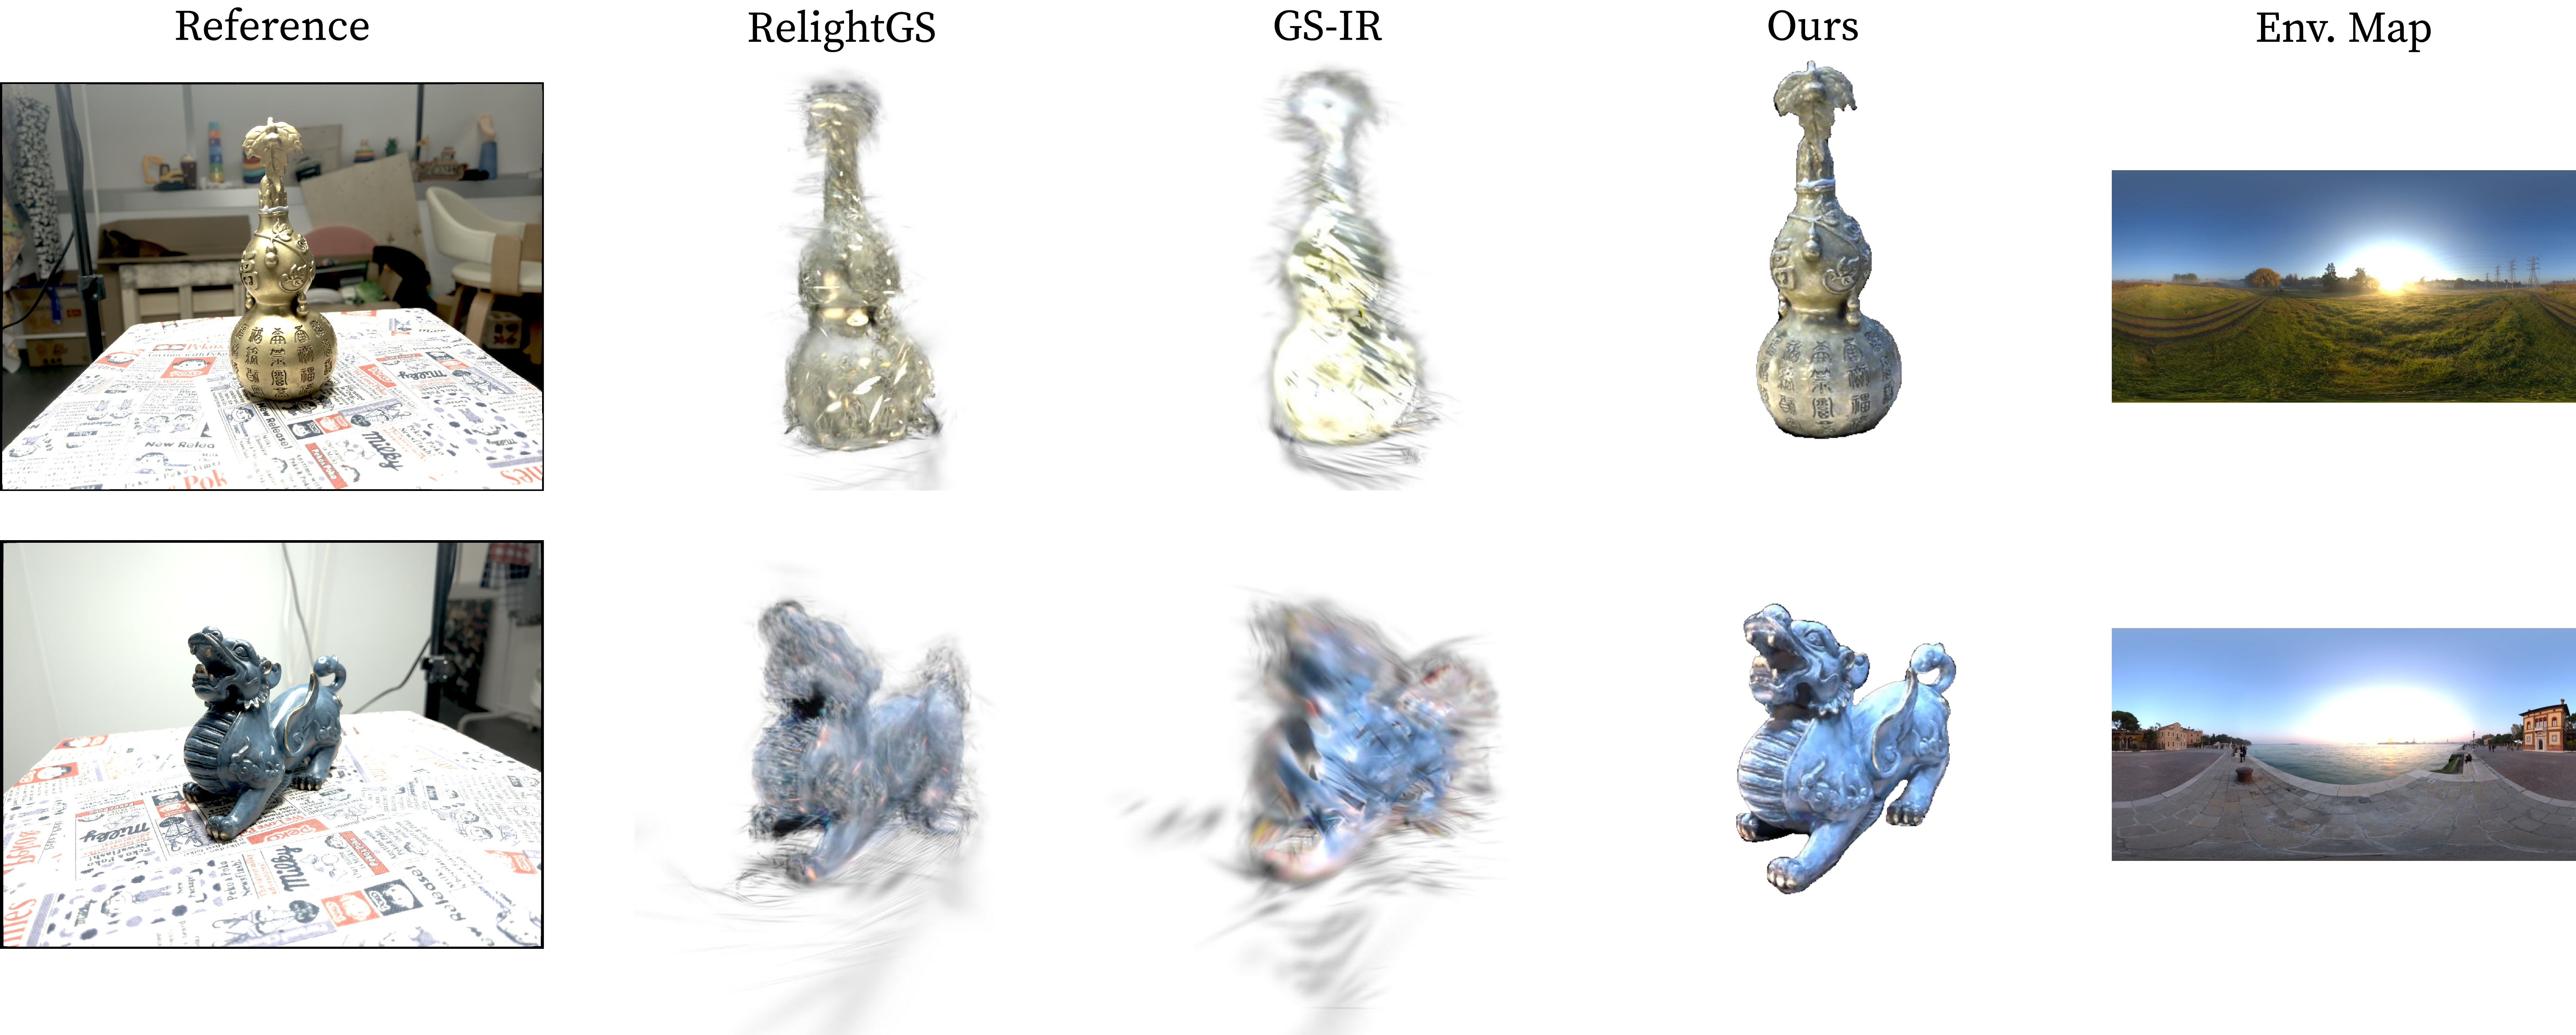}
%     \caption{Relighting Qualitative comparison on NeILF++ dataset.}
%     \label{fig:sup_neilfpp}
%     \vspace{-20pt}
% \end{figure*}

% \begin{figure*}[t]
%     \vspace{-20pt}
%     \centering
%     \includegraphics[width=0.95\textwidth]{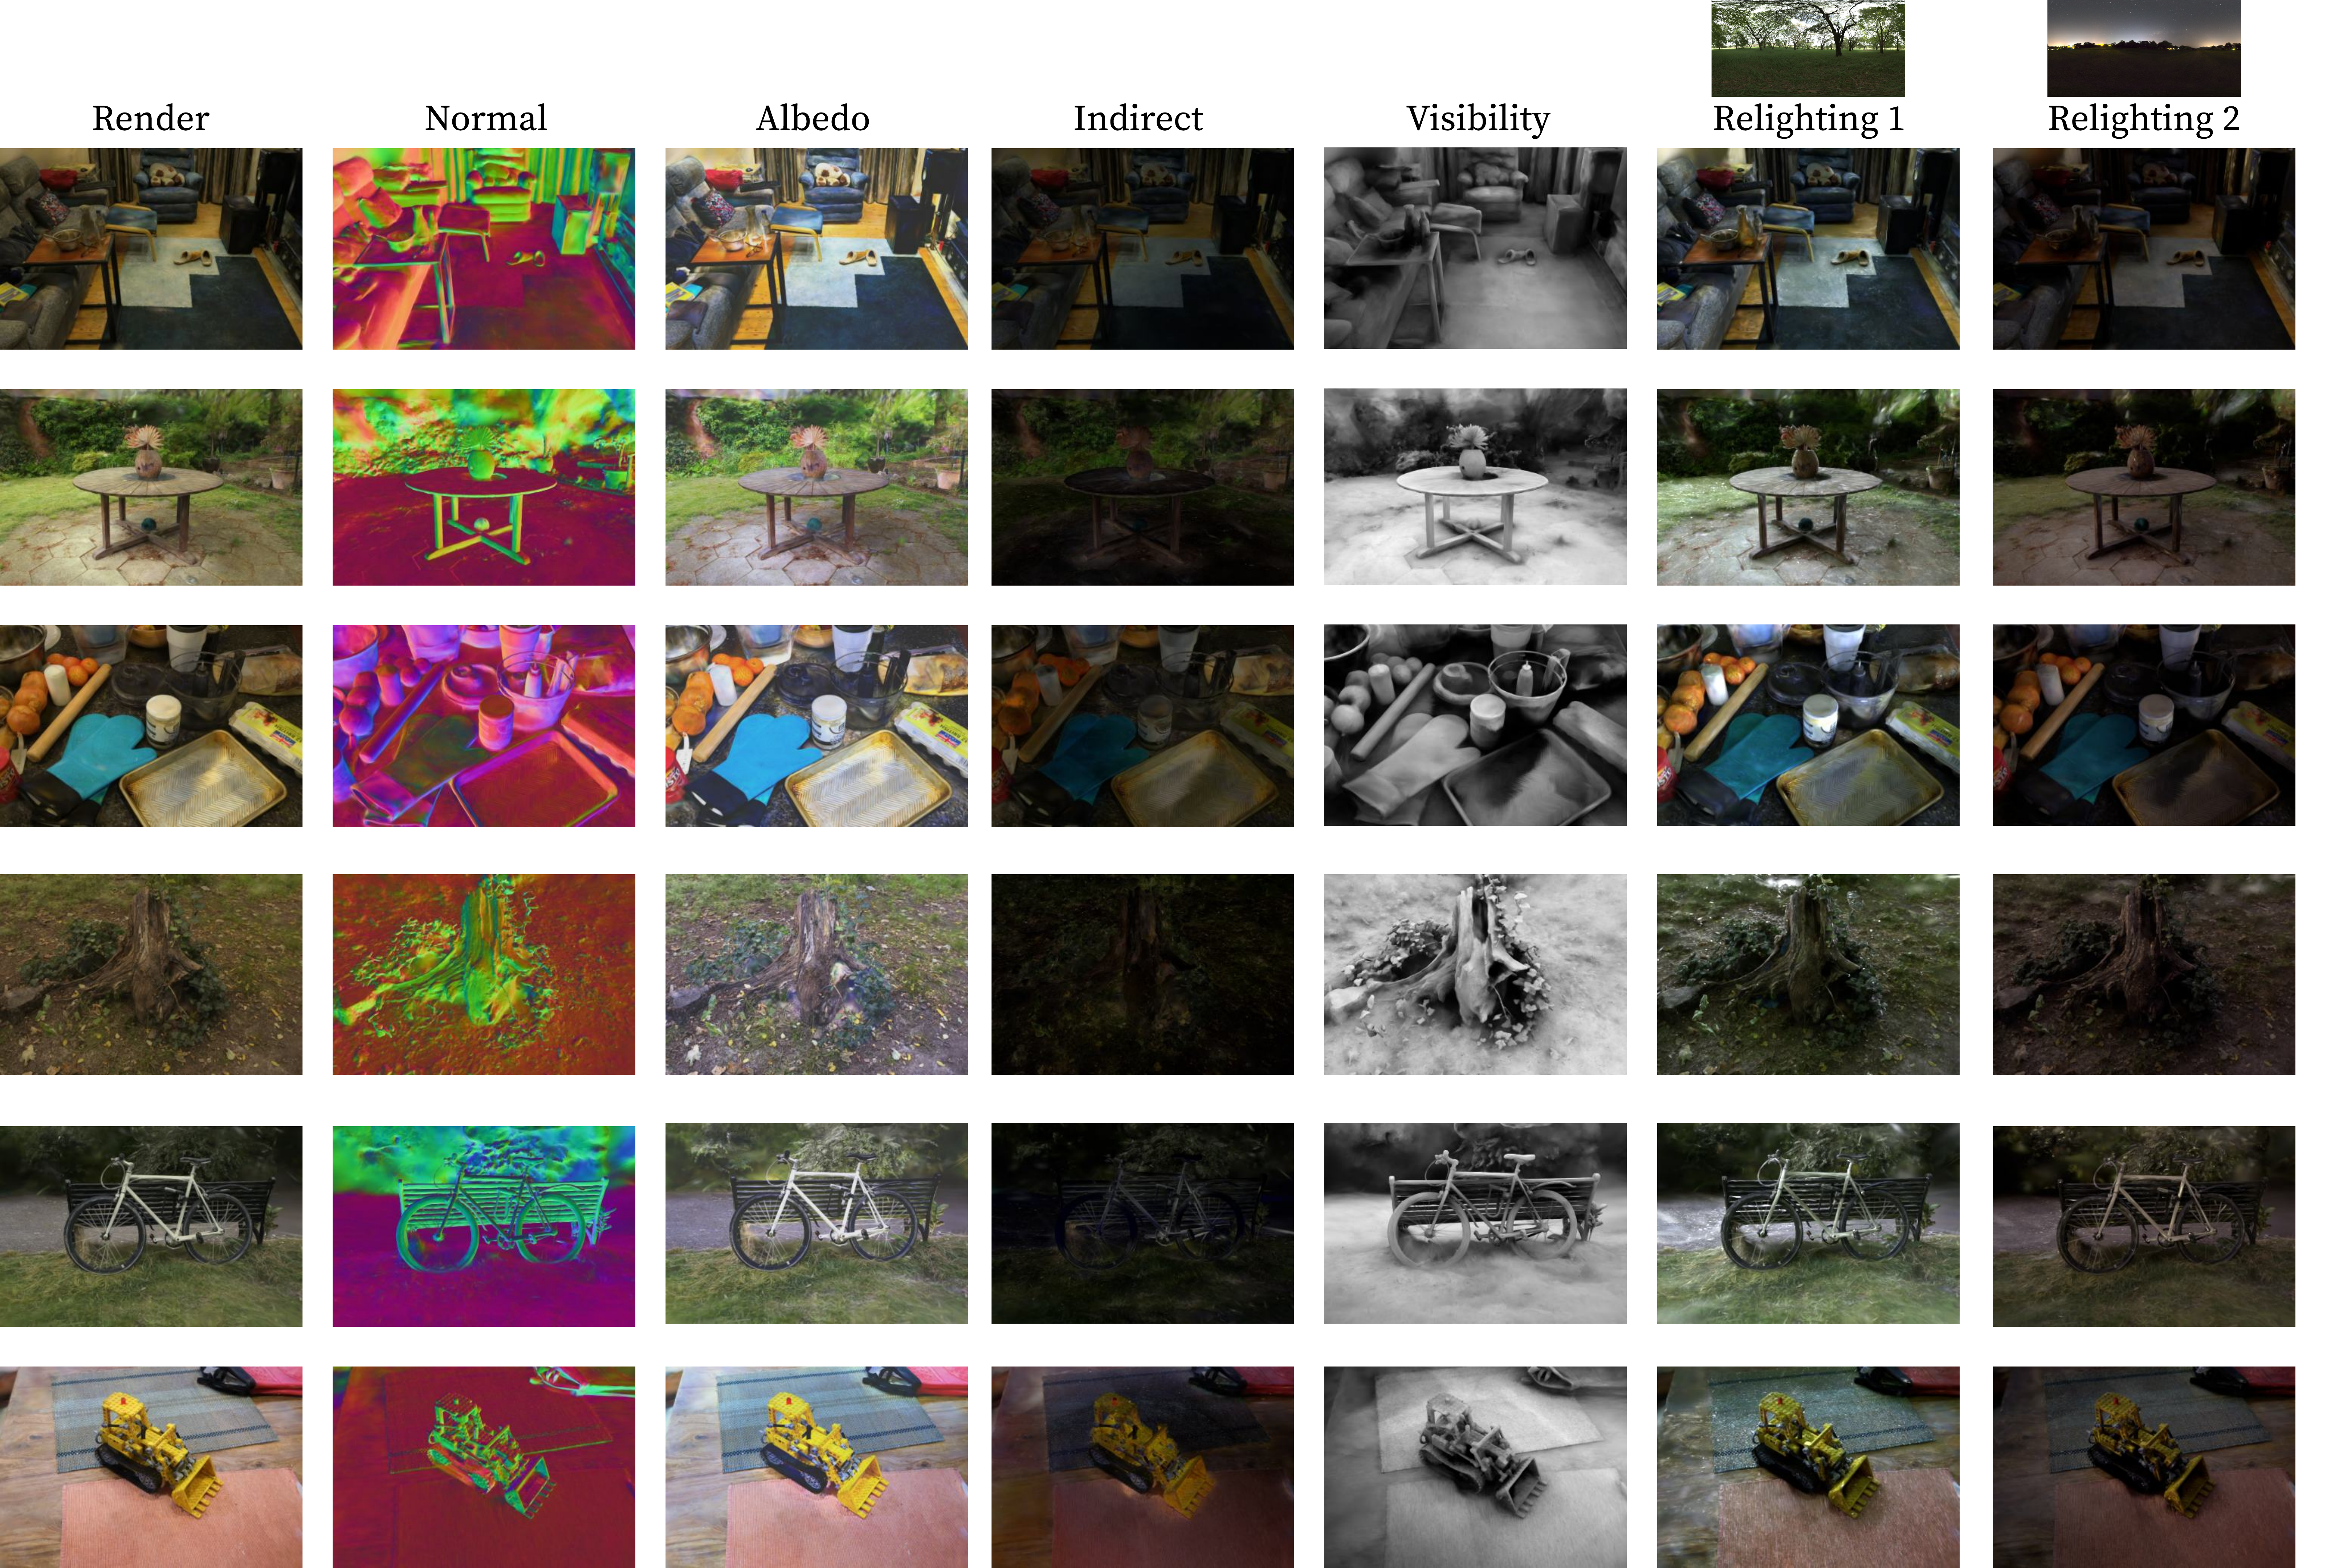}
%     \caption{Inverse rendering and relighting results on MipNeRF360 dataset.}
%     \label{fig:sup_mip}
%     \vspace{-20pt}
% \end{figure*}
\mycfiguret{sup_dtu}{sup_DTU.pdf}{Inverse rendering and relighting results on DTU dataset. }
\mycfiguret{sup_neilfpp}{sup_NeILF++.pdf}{Relighting Qualitative comparison on NeILF++ dataset. }
\mycfiguret{sup_mip}{sup_MipNeRF360.pdf}{Inverse rendering and relighting results on MipNeRF360 dataset. }
% \section{Rationale}
% \label{sec:rationale}
% % 
% Having the supplementary compiled together with the main paper means that:
% % 
% \begin{itemize}
% \item The supplementary can back-reference sections of the main paper, for example, we can refer to \cref{sec:intro};
% \item The main paper can forward reference sub-sections within the supplementary explicitly (e.g. referring to a particular experiment); 
% \item When submitted to arXiv, the supplementary will already included at the end of the paper.
% \end{itemize}
% % 
% To split the supplementary pages from the main paper, you can use \href{https://support.apple.com/en-ca/guide/preview/prvw11793/mac#:~:text=Delete%20a%20page%20from%20a,or%20choose%20Edit%20%3E%20Delete).}{Preview (on macOS)}, \href{https://www.adobe.com/acrobat/how-to/delete-pages-from-pdf.html#:~:text=Choose%20%E2%80%9CTools%E2%80%9D%20%3E%20%E2%80%9COrganize,or%20pages%20from%20the%20file.}{Adobe Acrobat} (on all OSs), as well as \href{https://superuser.com/questions/517986/is-it-possible-to-delete-some-pages-of-a-pdf-document}{command line tools}.

% P4RvyK7tTQUfuWm72Adp%jB6oPjH*!Ni
